# Supplementary material for: MultiGO: Towards Multi-level Geometry Learning for Monocular 3D Textured Human Reconstruction
Source: arXiv:2412.03103 source file (2024-12-04)
Supplement: Supplementary file 1 [file X_suppl.tex]

\clearpage
\setcounter{page}{1}
\maketitlesupplementary

\section{Implementation Details}
\subsection{Datasets}

The details of the three datasets used in our experiments are listed as follows, including THuman2.0, THuman3.0, and CustomHumans:
\begin{itemize}
    \item \textbf{THuman2.0}~\cite{tao2021function4d_thuman}: Thuman2.0 is a dataset with 525 high-resolution 3D human scans wearing over 150 different types of clothing. We use this dataset as our training data.
    \item \textbf{THuman3.0}~\cite{thuman3.0}: THuman3.0 is a dataset that contains over 20 combinations of human garments, each containing 15 to 35 high-quality human scans. In this paper, we select 60 scans for all of our experiments and ablation studies. In Table~\ref{thuman30samples}, we specifically display the test sample number we have selected.
    \item \textbf{CustomHumans}~\cite{ho2023customhuman}: CustomHumans is a dataset with 600 high-quality human scans of 80 subjects in over 100 garments and poses. Following the previous work SiTH~\cite{ho2024sith}, we selected 60 subjects for all of the experiments and ablation studies.
\end{itemize}
\subsection{Experimental Setting}
\myparagraph{Training} All experiments are conducted using four NVIDIA A800 GPUs. Our multimodal UNet is initialized with the pre-trained model from the work~\cite{tang2024lgm}. We set the input size of the single-view RGB images to 512x512 pixels and the Fourier expansion order ($q$) to 8. During training, we render human scans online using the official nvdiffrast library. We randomly sample 8 views to generate 8 RGB images, which are used to constrain the proposed Gaussian, and we then select one of these images as the input view, whose camera elevation and azimuth are set to 0,0. The learning rate for the AdamW~\cite{adamw} optimizer is set to  $5\times10^{-5}$. In training, we use the officially released fitting SMPL-X parameters~\cite{tao2021function4d_thuman} as input and the default disturbance value ($\alpha$) is set to 0.25. The pre-trained UNet of the wrinkle-level refinement module is from the work~\cite{unique3d}. Specifically, we freeze the VAE and CLIP image encoder and only update the UNet. All of the input images are rendered with nvdiffrast and resized to 512x512 pixels. We randomly selected 8 horizontal camera-rendered images and top and bottom camera-rendered images as our initialization inputs and de-noising conditions. During training, we set the de-noising step $k$ to 1. The learning rate of AdamW optimizer is set to $1\times10^{-5}$. All models are trained to converge.

\myparagraph{Inference} In inference, we estimate the SMPL-X parameters from the input single-view image. The output of our models is the 3D Gaussian representation, which is transformed
into the 3D mesh using the official script file provided by LGM~\cite{tang2024lgm}. During the refinement step, the coarse normal map $I_n$ in the input images are rendered online with nvdiffrast library while the RGB images $I_c$ are rendered from the output 3D Gaussian with diff-gaussian-rasterizer~\cite{3DGaussian}. During remeshing, we set the learning rate of the vertices optimizer to $0.3$ and the laplacian weight to $0.01$. We iteratively update the mesh for $100$ steps to obtain the refined mesh.

\subsection{CAPE dataset}
In this section, we clarify our decision to exclude the CAPE dataset~\cite{ma2020cape} as our test set. As highlighted in the appendix of SiTH~\cite{ho2024sith}, the CAPE dataset has several significant shortcomings. It features incomplete input images rendered from unprocessed point clouds, and the ground truth (GT) meshes are of low resolution, failing to accurately correspond to the input images. Additionally, the dataset suffers from limited diversity in human outfitting, as the majority of subjects are depicted in tight clothing such as t-shirts and shorts. We present some samples from the CAPE dataset in Figure~\ref{cape_images}. Given these limitations, we opted for higher-quality datasets to ensure an unbiased comparison of our method against the latest advancements in the field. Notably, we have identified recently updated datasets, including CustomsHumans~\cite{ho2023customhuman} and THuman3.0~\cite{thuman3.0}, which offer comprehensive, high-resolution input data and a wider variety of human attire. This choice not only enhances the validity of our comparisons but also reflects our commitment to using the most robust and diverse data available in our research.

\begin{figure*}[t!]
    \centering
    \includegraphics[width=0.87\linewidth]{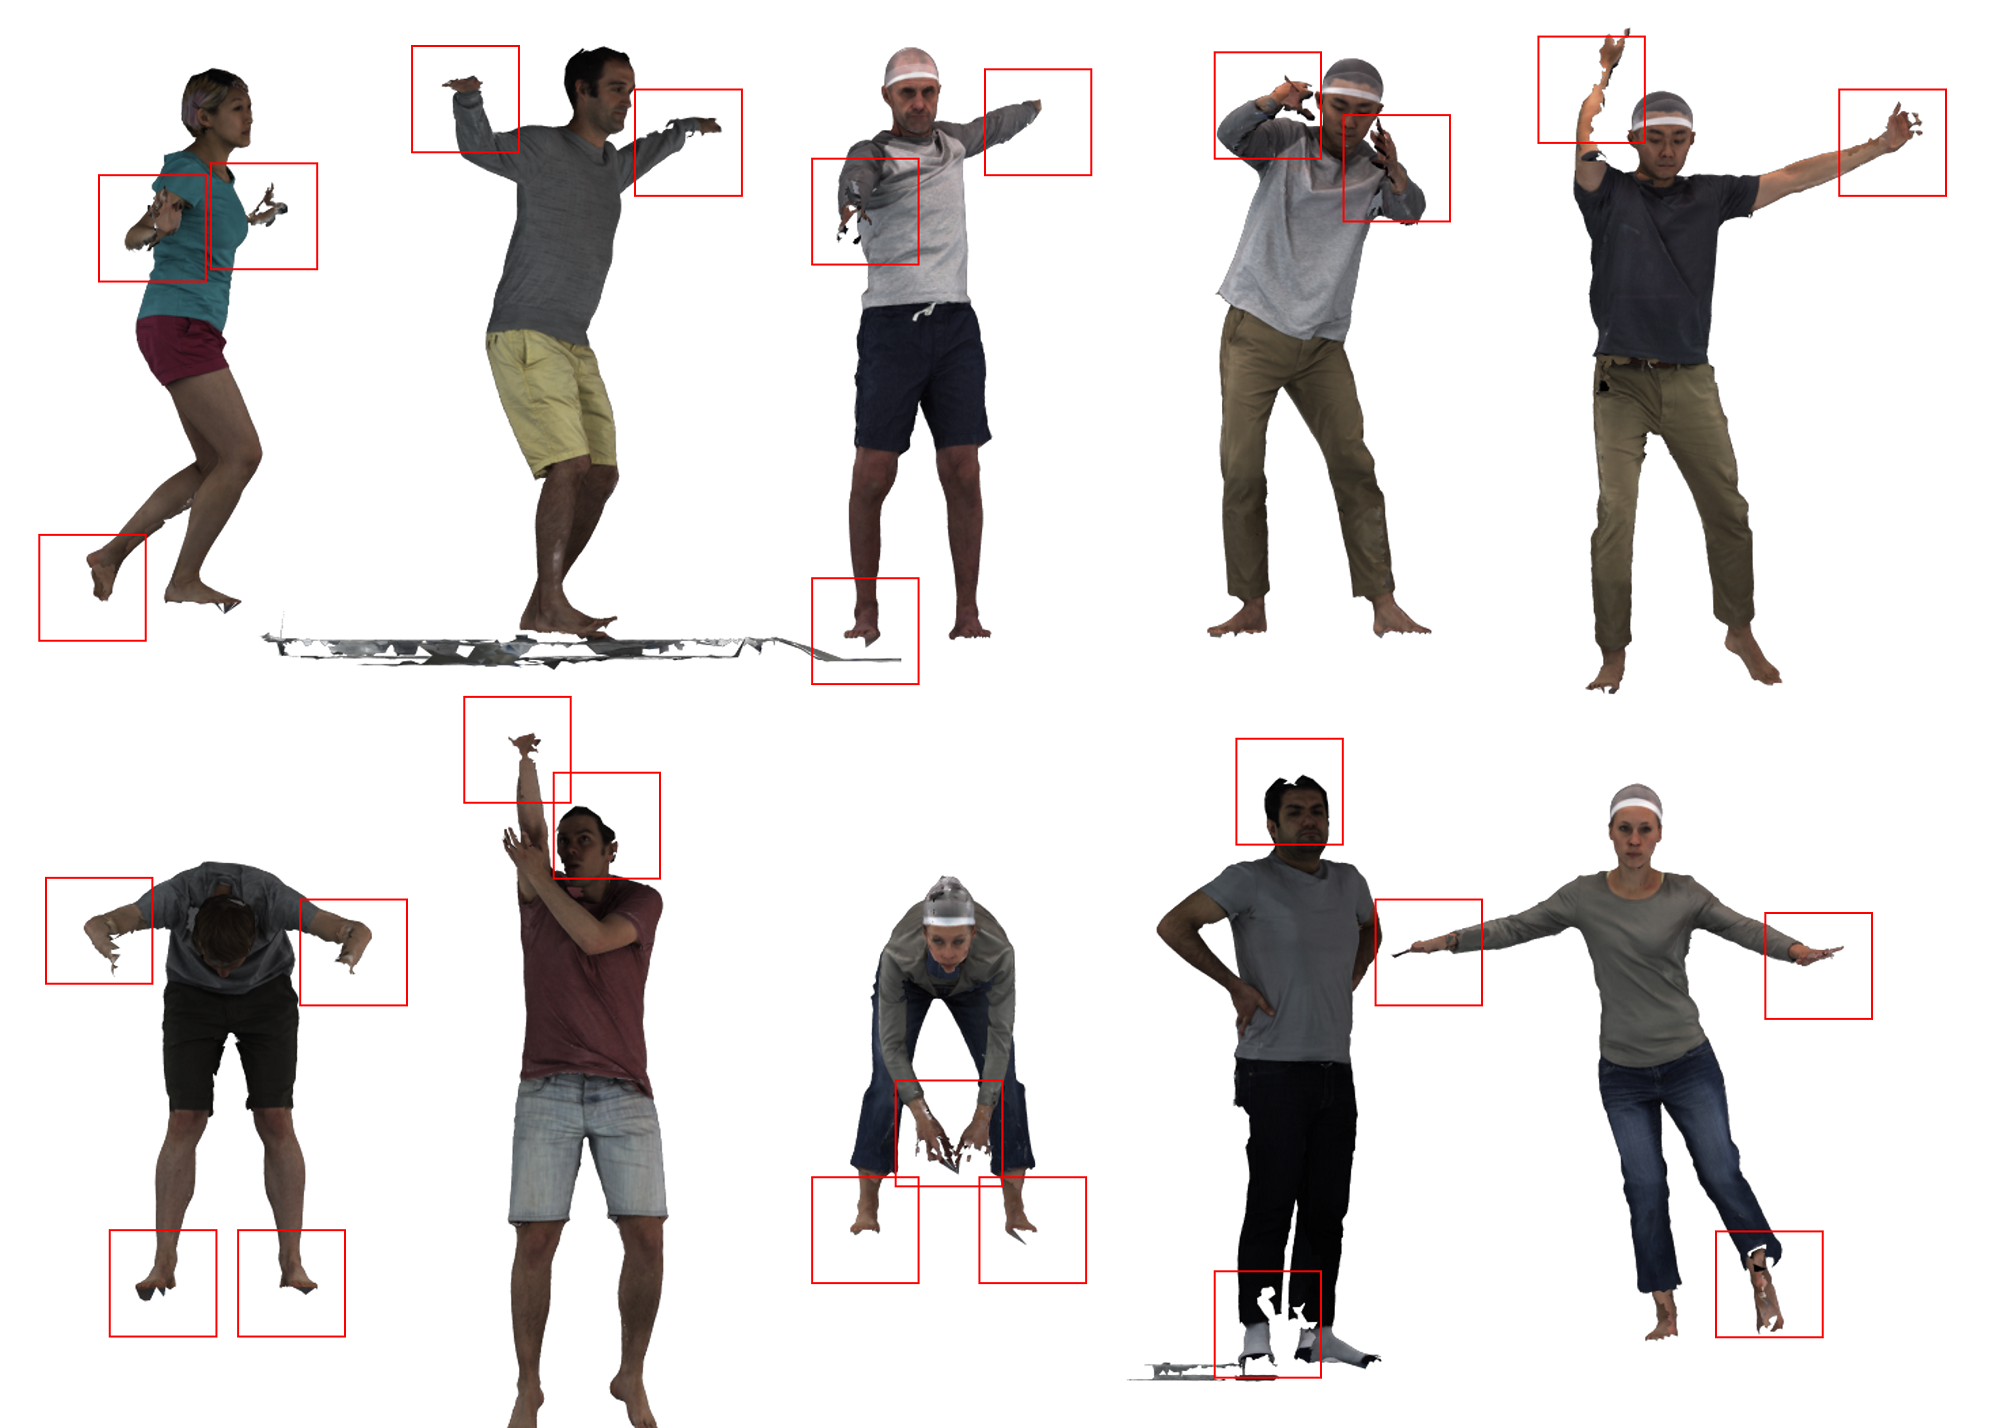}
        \vspace{-0.2cm}

    \caption{\textbf{Samples from the CAPE test set which contain noticeable defects.} We present some input images from the CAPE test set intuitively. From the displayed image, we can see significant issues with the quality of the input image provided by CAPE. Specifically, there are obvious defects in the characters' palms, feet, and head areas. Therefore, to reasonably evaluate the comparison with SOTA methods, we chose the latest and higher quality CustomsHumans and THuman3.0 as our test set.}
    \label{cape_images}
            \vspace{-0.4cm}
\end{figure*}

\begin{figure*}[t!]
    \centering
    \includegraphics[width=0.87\linewidth]{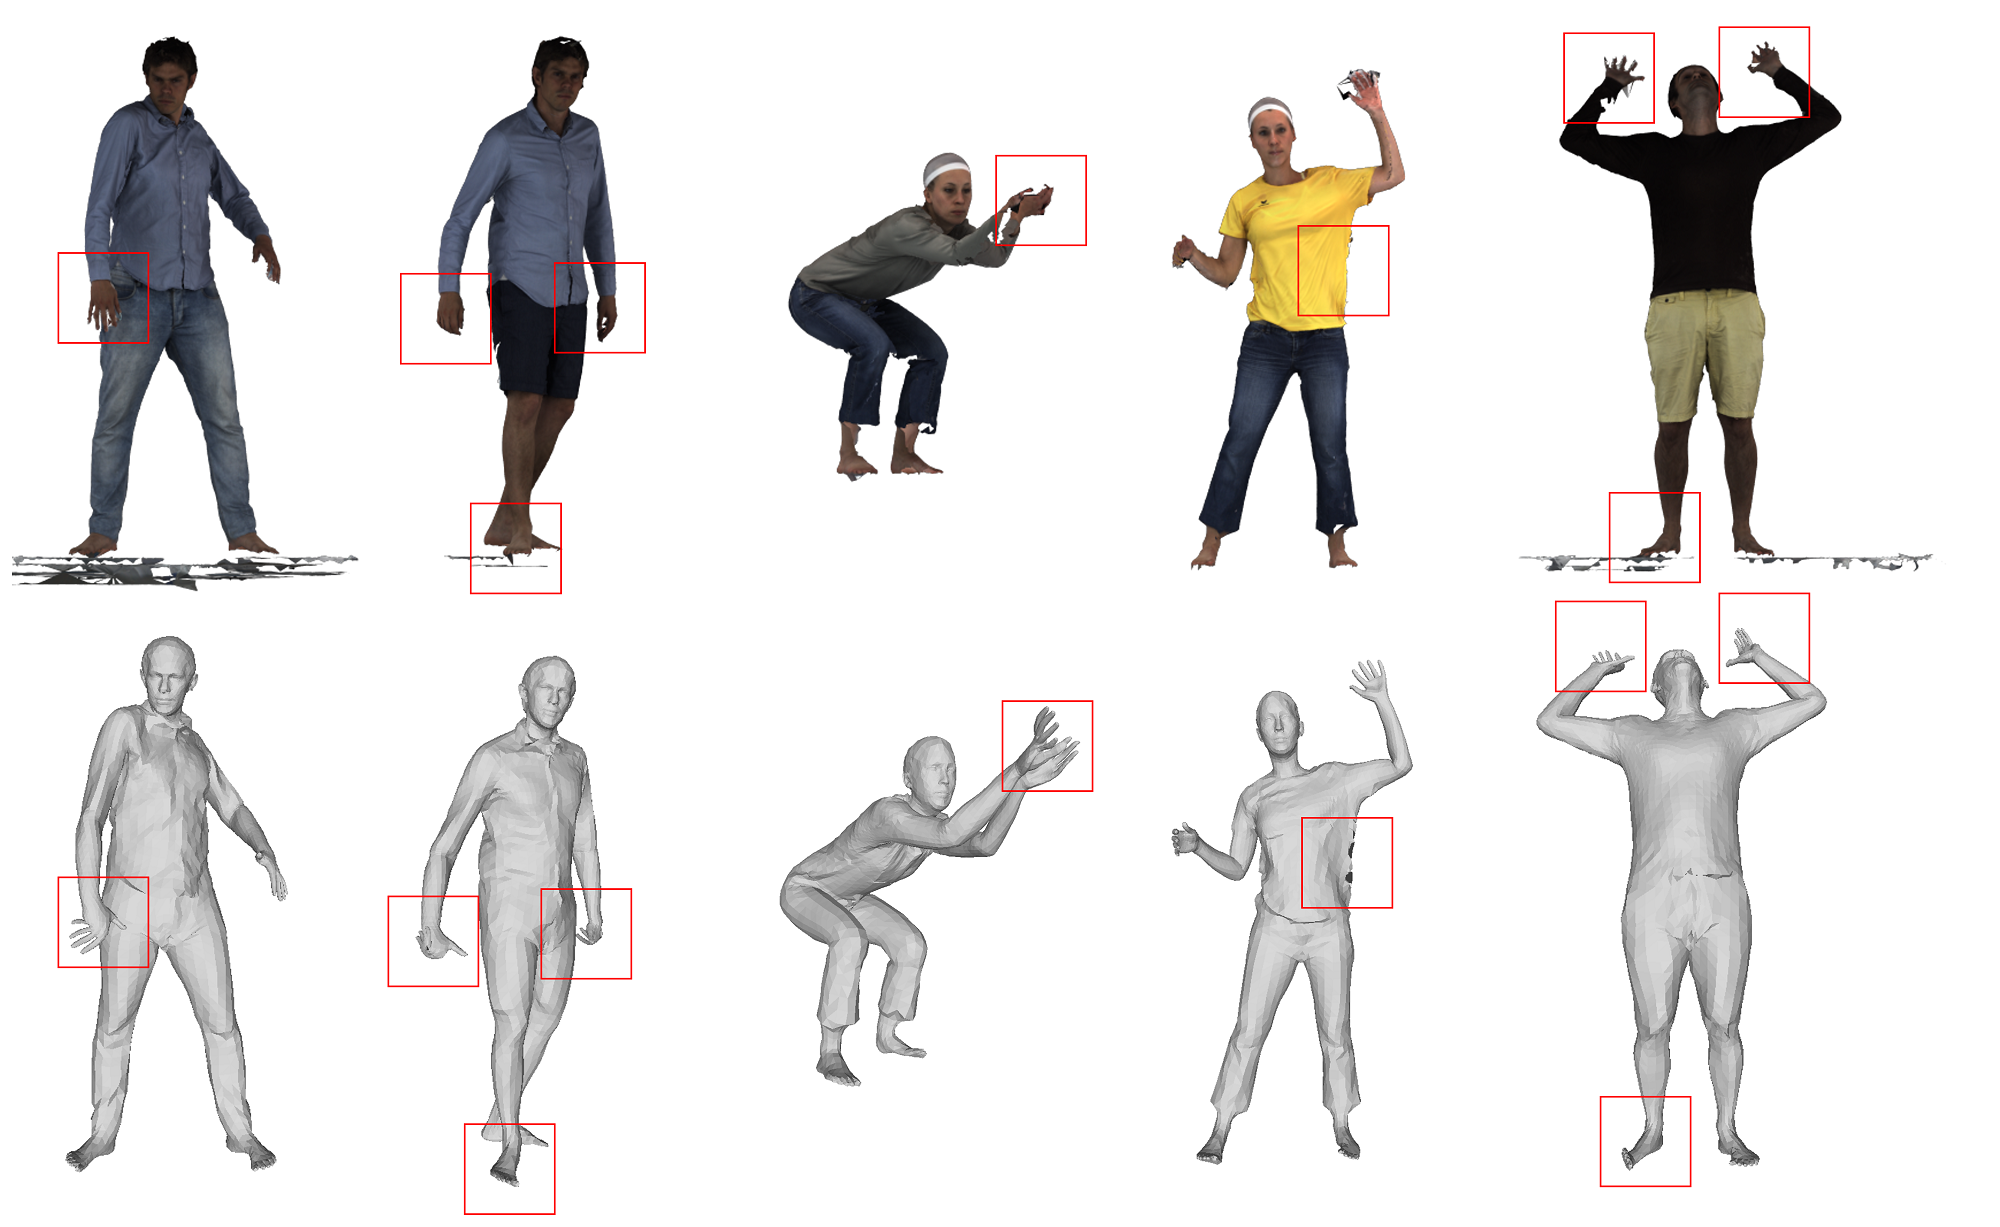}
        \vspace{-0.4cm}

    \caption{\textbf{Samples from the CAPE test set.} Comparing with the input images, it can be found that these GT meshes do not fully correspond to them. For example, in the palms and feet, GT meshes will produce varying degrees of distortion}
    \label{cape_images}
            \vspace{-0.4cm}
\end{figure*}

\section{More Experimental Results}
\subsection{Visualization on Ablation Study}

\begin{figure*}[t!]
    \centering
    \includegraphics[width=0.87\linewidth]{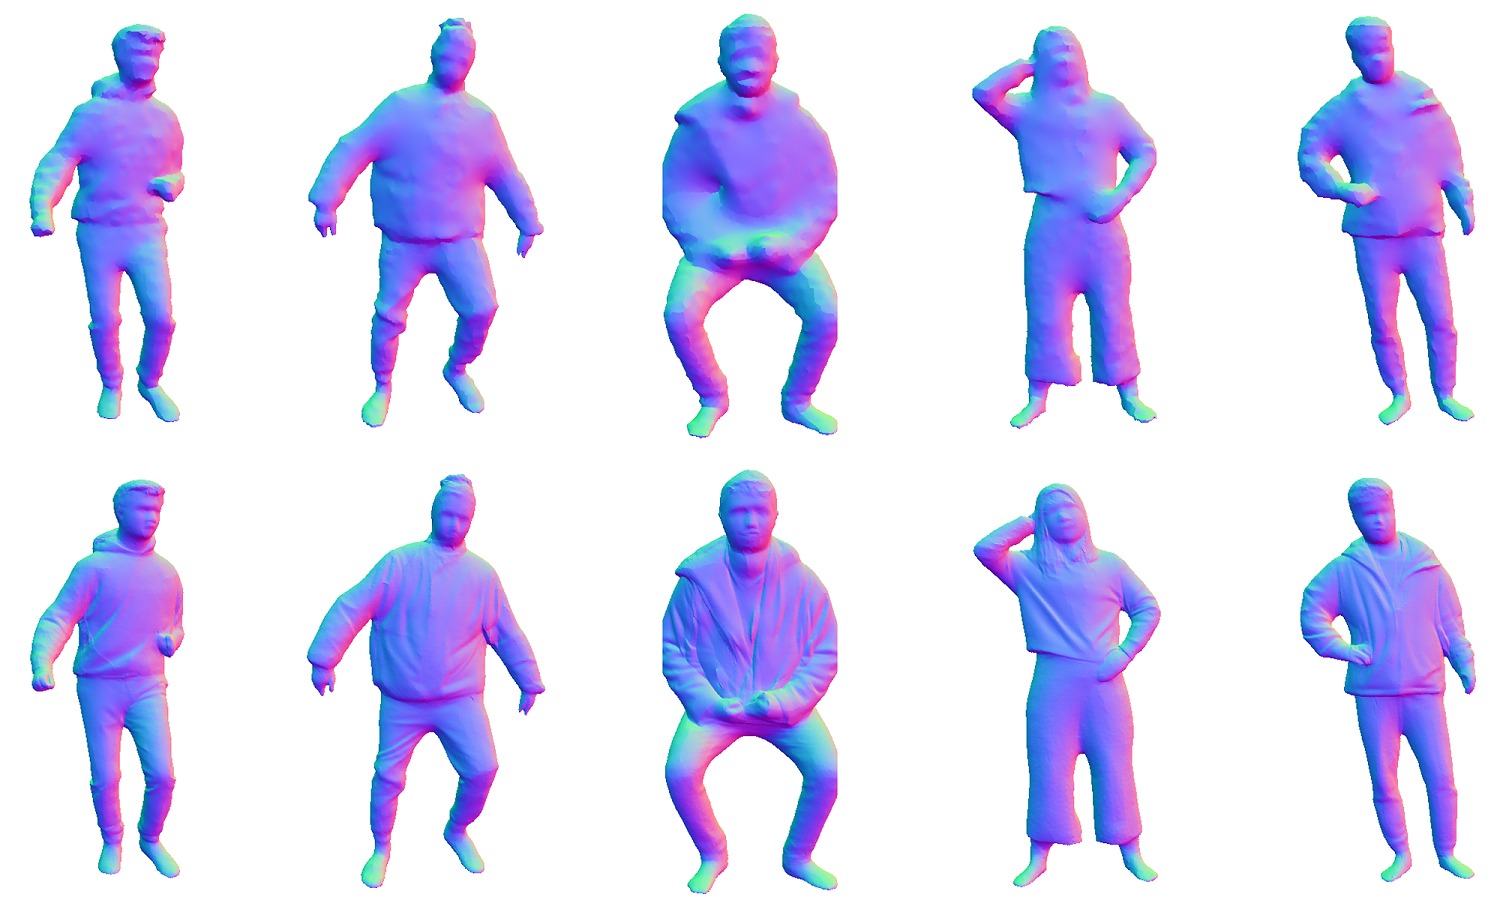}
        \vspace{-0.2cm}

    \caption{\textbf{More examples to illustrate the effectiveness of the proposed WLR module.} The first row shows the normal map rendered from the mesh before the introduction of the WLR module, and the second row shows the normal map rendered by the mesh after the introduction of the WLR module.}
    \label{refined_supp1}
            \vspace{-0.4cm}
\end{figure*}

\begin{figure*}[t!]
    \centering
    \includegraphics[width=0.87\linewidth]{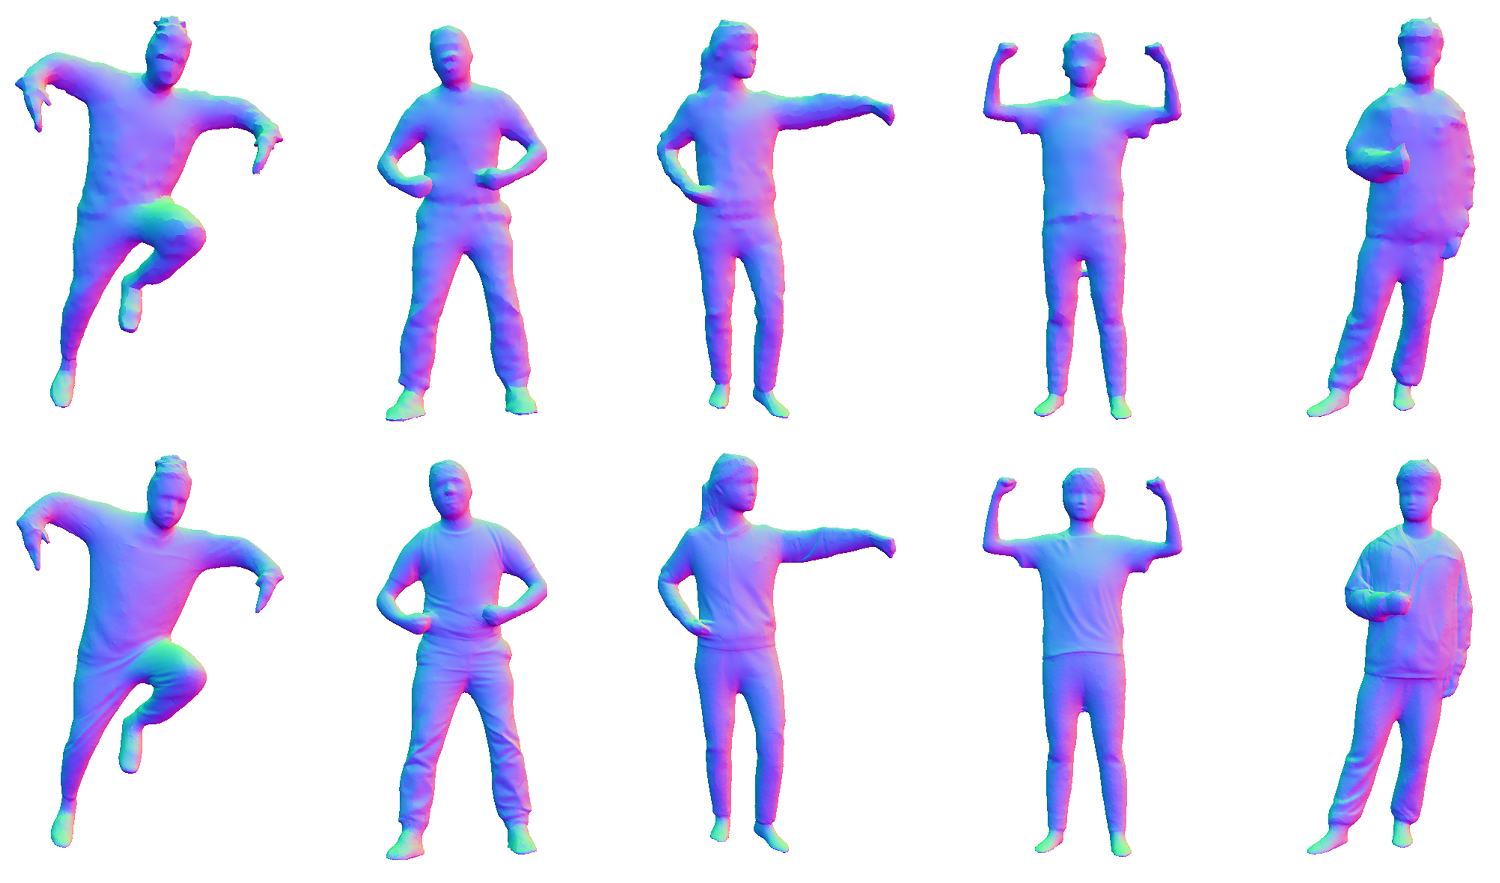}
        \vspace{-0.2cm}

    \caption{\textbf{More examples to illustrate the effectiveness of the proposed WLR module.} The first row shows the normal map rendered from the mesh before the introduction of the WLR module, and the second row shows the normal map rendered by the mesh after the introduction of the WLR module.}
    \label{refined_supp2}
            \vspace{-0.4cm}
\end{figure*}

\begin{figure*}[t!]
    \centering
    \includegraphics[width=0.87\linewidth]{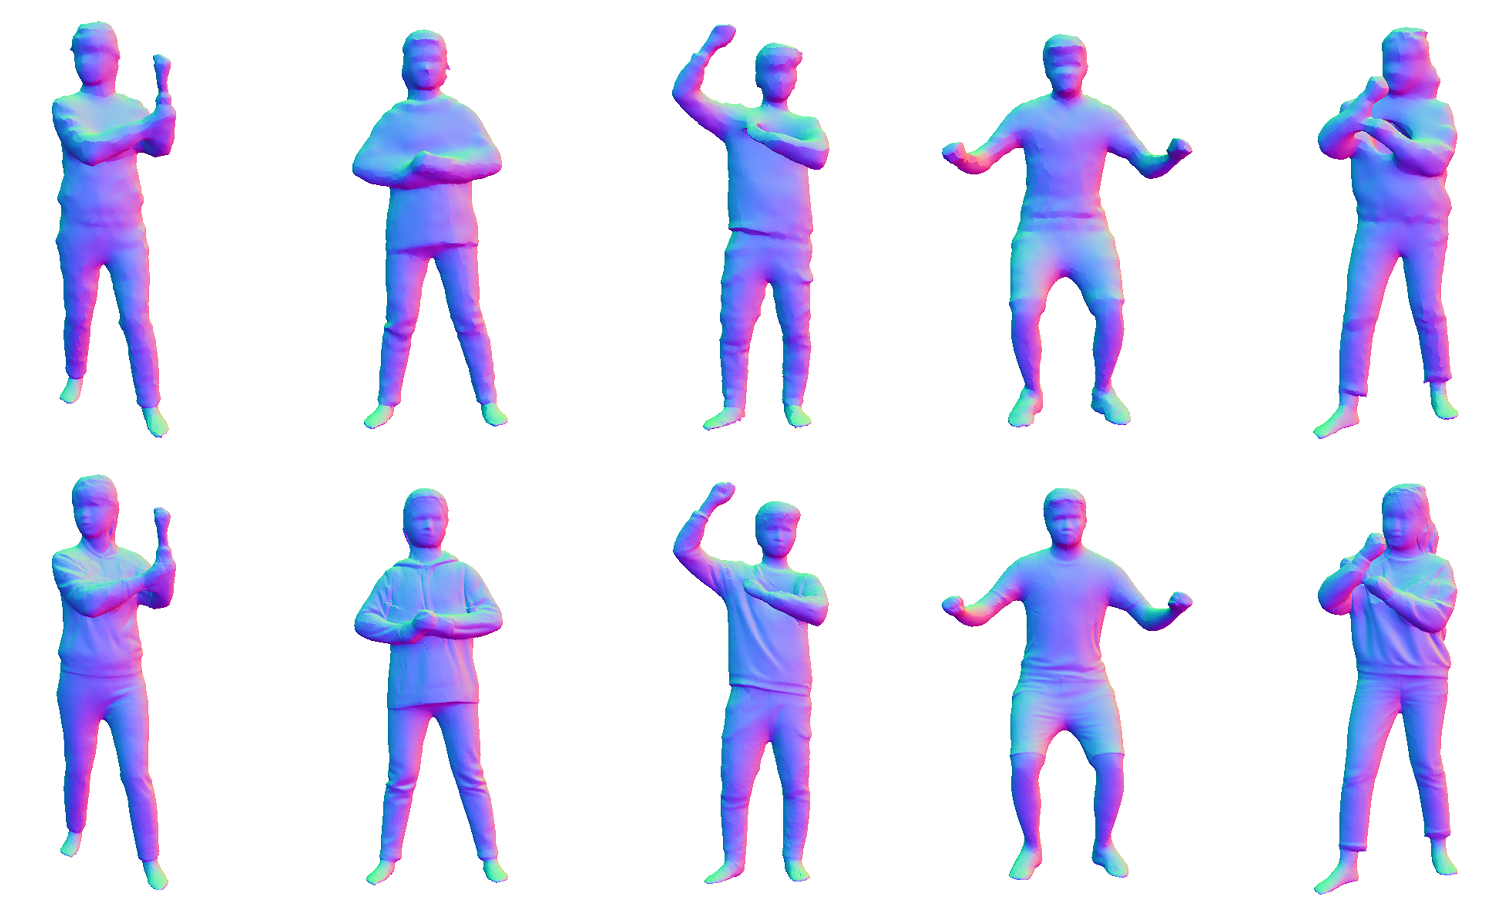}
        \vspace{-0.2cm}

    \caption{\textbf{More examples to illustrate the effectiveness of the proposed WLR module.} The first row shows the normal map rendered from the mesh before the introduction of the WLR module, and the second row shows the normal map rendered by the mesh after the introduction of the WLR module.}
    \label{refined_supp3}
            \vspace{-0.4cm}
\end{figure*}

\begin{figure*}[t!]
    \centering
    \includegraphics[width=1\linewidth]{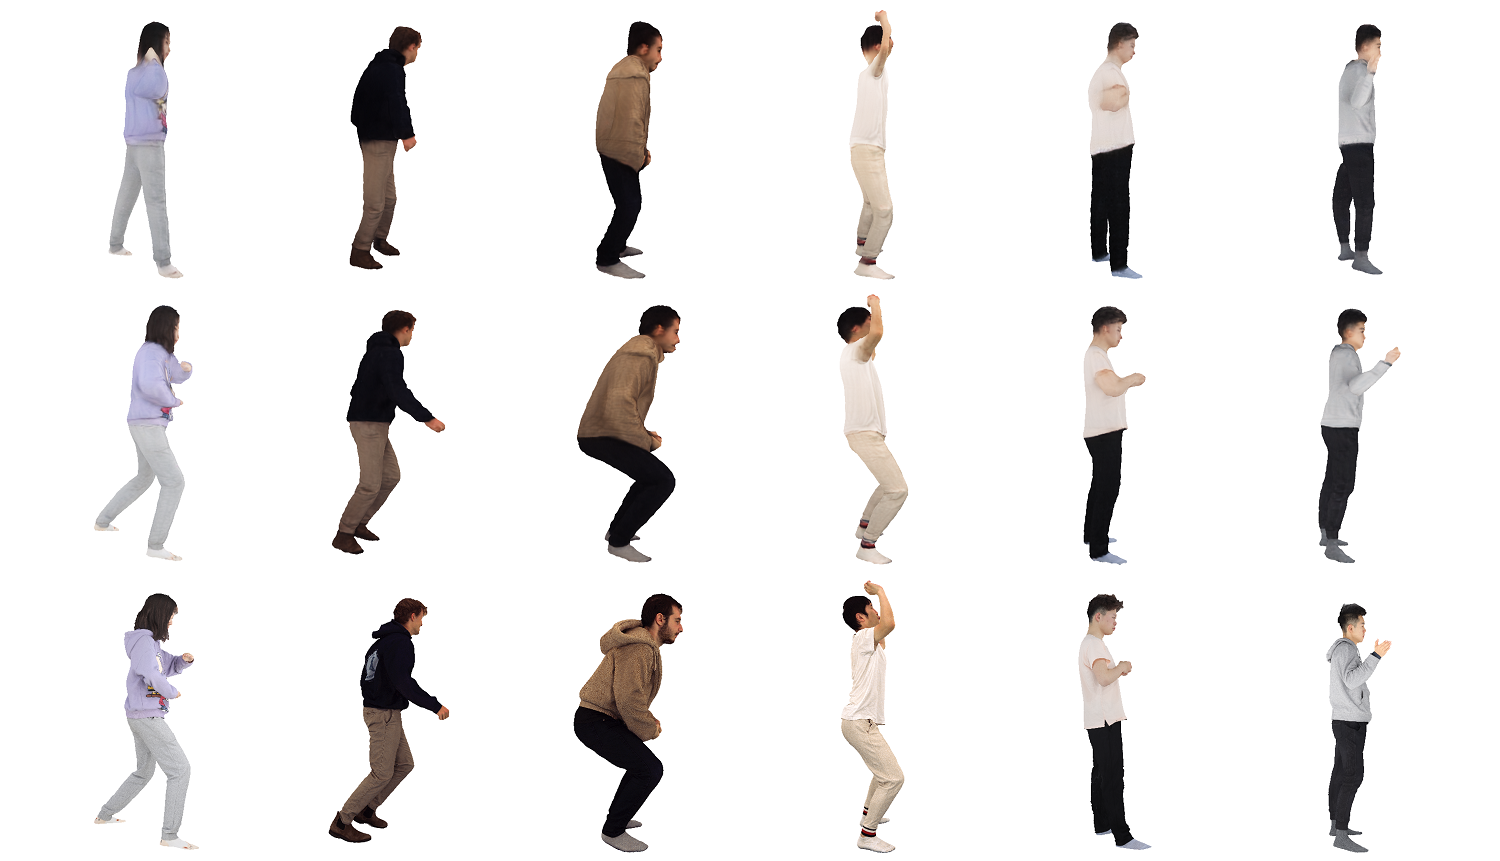}
        \vspace{-0.2cm}

    \caption{\textbf{More examples to illustrate the effectiveness of the proposed SLE module.} The first row shows the side rendering of the reconstructed human before the introduction of the SLE module. The second row shows the side rendering of the reconstructed human after the introduction of the SLE module. The third row shows the side the rendering of the ground truth.}
    \label{SLE_supp}
            \vspace{-0.4cm}
\end{figure*} 

\begin{table*}
\begin{center}
\centering
    \scalebox{0.7}{
    \begin{tabular}{@{\extracolsep{\fill}}ccc|ccc}
    \toprule
    Scan ID in our Exp. & Scan ID in THuman3.0 & Subject ID & Scan ID in our Exp. & Scan ID in THuman3.0 & Subject ID \\
    \midrule
       1                & 00001\_0033 & 1 & 31   & 00008\_0042 & 11 \\
       2                & 00001\_0069 & 1 & 32   & 00008\_0046 & 11 \\
       3                & 00001\_0070 & 1 & 33   & 00008\_0032 & 11 \\
       4                & 00001\_0047 & 2 & 34   & 00008\_0049 & 12 \\
       5                & 00001\_0049 & 2 & 35   & 00008\_0052 & 12 \\
       6                & 00001\_0052 & 2 & 36   & 00008\_0057 & 12 \\
       7                & 00003\_0003 & 3 & 37   & 00023\_0012 & 13 \\
       8                & 00003\_0013 & 3 & 38   & 00023\_0080 & 13 \\
       9                & 00003\_0018 & 3 & 39   & 00023\_0008 & 13 \\
       10               & 00003\_0021 & 4 & 40   & 00024\_0014 & 14 \\
       11               & 00003\_0035 & 4 & 41   & 00024\_0023 & 14 \\
       12               & 00003\_0036 & 4 & 42   & 00024\_0025 & 14 \\
       13               & 00004\_0007 & 5 & 43   & 00024\_0039 & 15 \\
       14               & 00004\_0014 & 5 & 44   & 00024\_0043 & 15 \\
       15               & 00004\_0022 & 5 & 45   & 00024\_0052 & 15 \\
       16               & 00005\_0022 & 6 & 46   & 00025\_0004 & 16 \\
       17               & 00005\_0023 & 6 & 47   & 00025\_0005 & 16 \\
       18               & 00005\_0005 & 6 & 48   & 00025\_0006 & 16 \\
       19               & 00005\_0042 & 7 & 49   & 00026\_0026 & 17 \\
       20               & 00005\_0045 & 7 & 50   & 00026\_0034 & 17 \\
       21               & 00005\_0048 & 7 & 51   & 00026\_0039 & 17 \\
       22               & 00006\_0022 & 8 & 52   & 00027\_0005 & 18 \\
       23               & 00006\_0006 & 8 & 53   & 00027\_0032 & 18 \\
       24               & 00006\_0007 & 8 & 54   & 00027\_0027 & 18 \\
       25               & 00007\_0009 & 9 & 55   & 00028\_0034 & 19 \\
       26               & 00007\_0021 & 9 & 56   & 00028\_0025 & 19 \\
       27               & 00007\_0030 & 9 & 57   & 00028\_0020 & 19 \\ 
       28               & 00008\_0005 & 10 & 58  & 00060\_0018 & 20 \\
       29               & 00008\_0013 & 10 & 59  & 00060\_0010 & 20 \\    
       30               & 00008\_0044 & 10 & 60  & 00060\_0028 & 20 \\
    \bottomrule
    \end{tabular}
}
\caption{Details about the 60 scans from THuman3.0 used in our experiment. We report the Scan ID in our experiment its corresponding ID in Thuman3.0 and the subject ID. \label{thuman30samples}}
\end{center}
\end{table*}

\myparagraph{Additional Examples Demonstrating the Effectiveness of the Proposed WLR Module} Figures~\ref{refined_supp1},~\ref{refined_supp2}, and~\ref{refined_supp3} provide further insights into the impact of the Wrinkle-Level Refinement (WLR) module by comparing results before and after its implementation. The results clearly illustrate that the WLR module significantly enhances the geometric quality of the reconstructed mesh, particularly in capturing intricate details such as clothing wrinkles and facial features.

\myparagraph{Additional Examples Demonstrating the Effectiveness of the Proposed SLE Module} Figure~\ref{SLE_supp} presents additional results that highlight the effects of incorporating the Skeleton-Level Enhancement (SLE) module. The comparison reveals the SLE module effectively aids in reconstructing the target human geometry, resulting in a reconstructed mesh that closely resembles the ground truth mesh.
